# Supplementary material for: ReIFE: Re-evaluating Instruction-Following Evaluation
Source: arXiv:2410.07069 source file (2024-10-09)
Supplement: Supplementary file 1 [file Appendix_case_study_llama3_70b.tex]

\section{Case Study}
\label{appx_case_study_llama3_70b}

\begin{figure}[t!]
  \centering
  \includegraphics[width=1.0\textwidth]{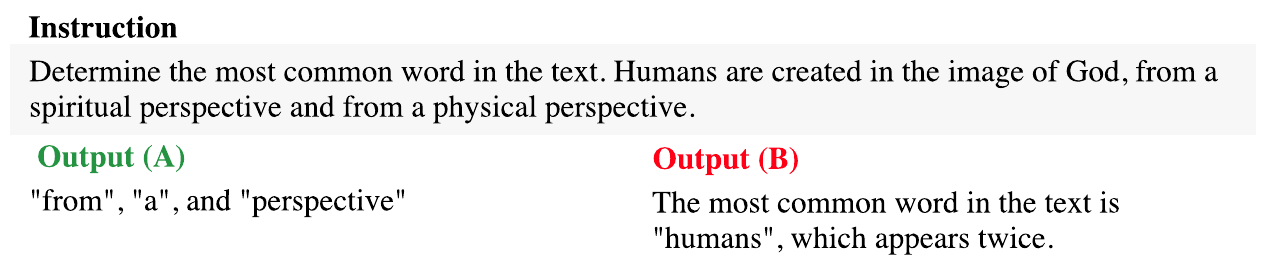}
  \label{fig:appx_case_70b_mtb_data}
\end{figure}

\begin{figure}[t!]
  \centering
  \includegraphics[width=1.05\textwidth]{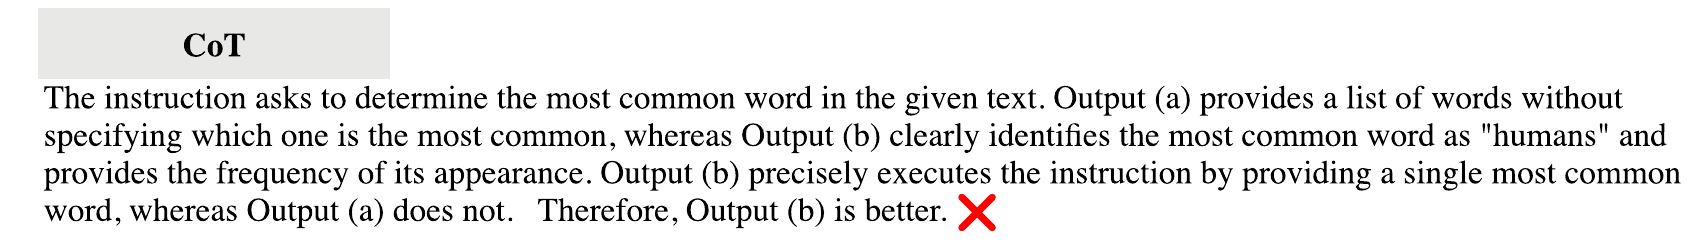}
  \label{fig:appx_case_70b_mtb_cot}
\end{figure}
\begin{figure}[t!]
  \centering
  \includegraphics[width=1.05\textwidth]{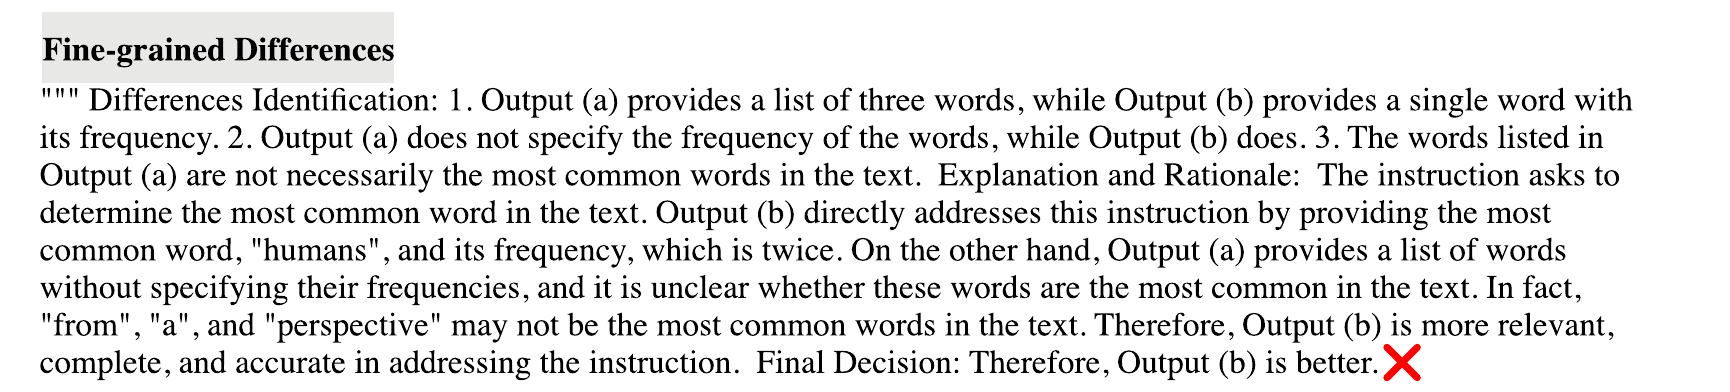}
  \label{fig:appx_case_70b_mtb_fine}
\end{figure}
\begin{figure}[t!]
  \centering
  \includegraphics[width=1.05\textwidth]{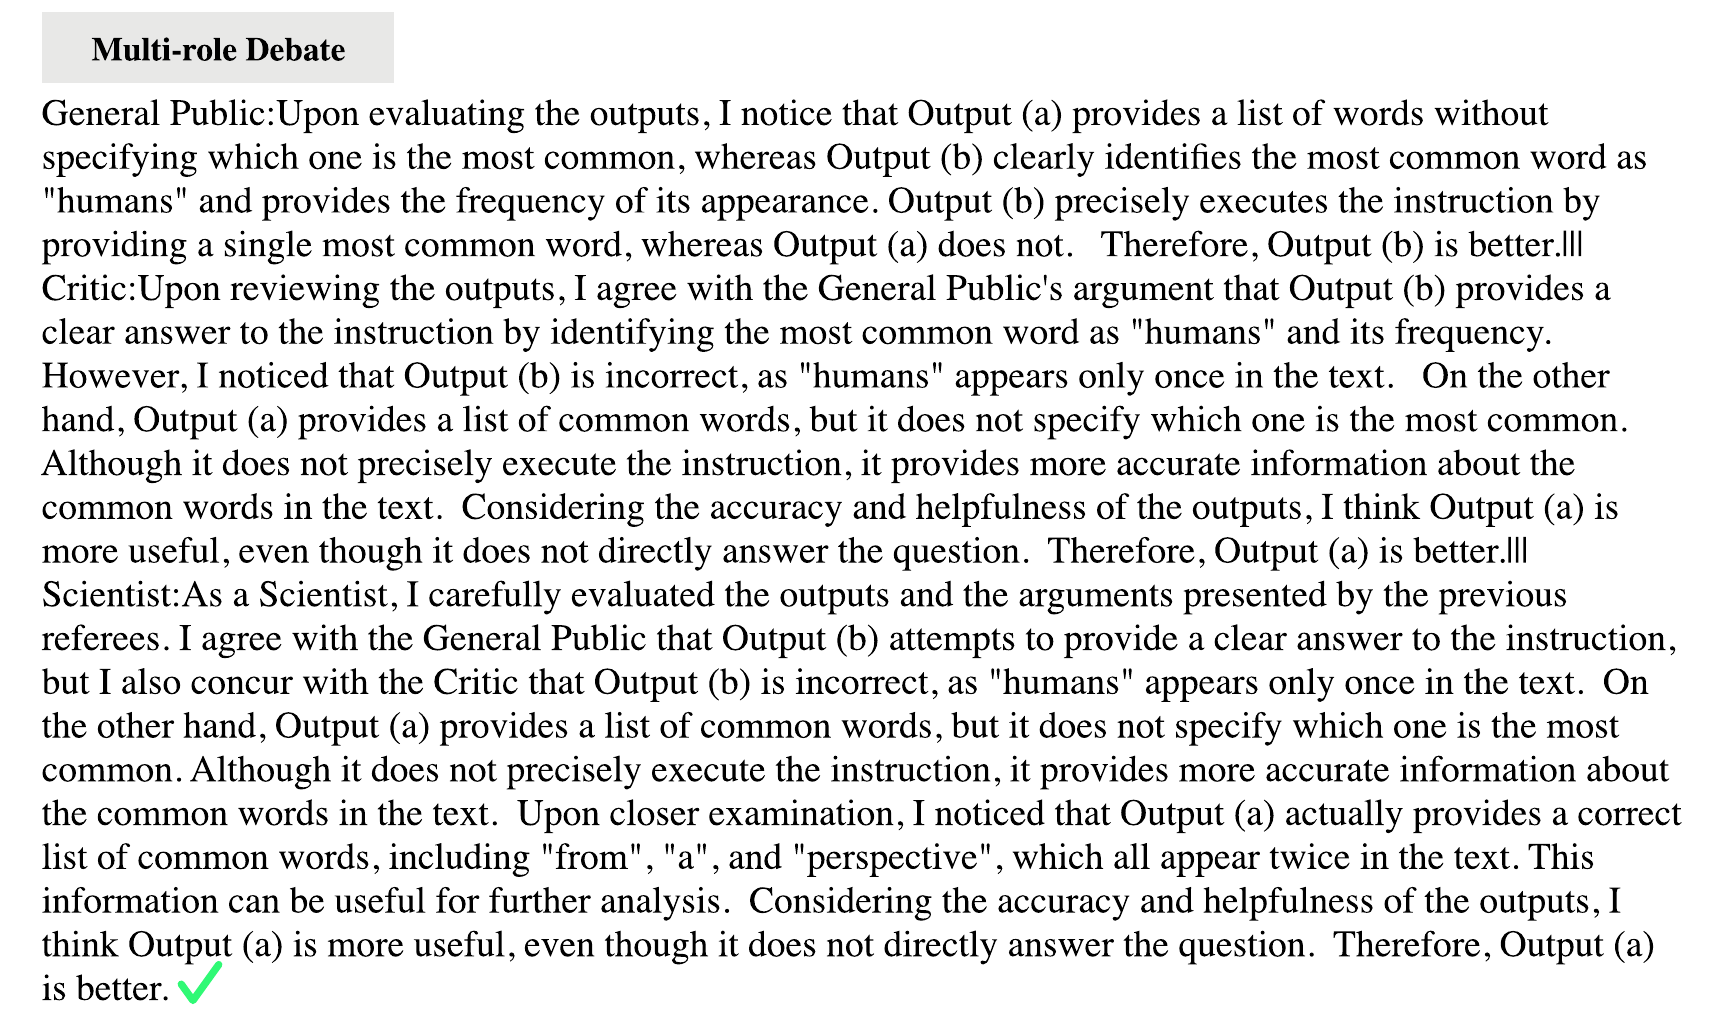}
  \label{fig:appx_case_70b_mtb_multi_role}
\end{figure}

\begin{figure}[t!]
  \centering
  \includegraphics[width=1.05\textwidth]{figures/8.pdf}
  \label{fig:appx_case_70b_mtb_aspect_final}
\end{figure}
