# Supplementary material for: ReIFE: Re-evaluating Instruction-Following Evaluation
Source: arXiv:2410.07069 source file (2024-10-09)
Supplement: Supplementary file 3 [file Appendix_model_registry.tex]

\section{Model Details}
\label{appx_model_details}
We provide brief descriptions for the 32 LLMs adopted in this study in Table~\ref{tab:appx_model_registry}.

\input{tables/model_registry}
